# Supplementary material for: Estimating the Sizes of Binary Error-Correcting Constrained Codes
Source: arXiv:2301.05098 source file (2023-04-19)
Supplement: Supplementary file 1 [file supplement-v1.pdf]

# Supplement to: Estimating the Sizes of Binary Error-Correcting Constrained Codes

V. Arvind Rameshwar, *Student Member, IEEE,*

and Navin Kashyap, *Senior Member, IEEE*

## I. On the Weight Distribution of Constrained Sequences in $\mathbb{F}_2^n$

Suppose that we are interested in computing the weight distribution of words in $\{0,1\}^n$ that lie in a (constrained) set $\mathcal{A} \subseteq \{0,1\}^n$. Let $a_{i,\mathcal{A}}$ denote the number of constrained words of weight $i \in [0:n]$ and recall the definition of the $i^{\text{th}}$-Krawtchouk polynomial $K_i^{(n)}$, for a given blocklength $n$, where $K_i^{(n)}(z) = \sum_{\ell=0}^{i}(-1)^\ell \binom{z}{\ell}\binom{n-z}{i-\ell}$, and the notation $W_i = \{\mathbf{x} \in \{0,1\}^n : w(\mathbf{x}) = i\}$. The following theorem then holds true:

**Theorem I.1.** *The weight distribution of sequences that lie in a set $\mathcal{A} \subseteq \{0,1\}^n$ obeys*

$$a_{i,\mathcal{A}} = \sum_{j=0}^{n} K_i^{(n)}(j) \cdot \sum_{\mathbf{s}:\ w(\mathbf{s})=j} \widehat{\mathbb{1}_{\mathcal{A}}}(\mathbf{s}), \quad i \in [0:n].$$

*Proof.* The proof is again a simple application of Plancherel's Theorem. Observe that

$$\begin{aligned} a_{i,\mathcal{A}} &= \sum_{\mathbf{x}\in\mathcal{A}} \mathbb{1}_{W_i}(\mathbf{x}) \\ &= \sum_{\mathbf{x}\in\{0,1\}^n} \mathbb{1}_{W_i}(\mathbf{x}) \cdot \mathbb{1}_{\mathcal{A}}(\mathbf{x}) \\ &= 2^n \cdot \sum_{\mathbf{s}\in\{0,1\}^n} \widehat{\mathbb{1}_{W_i}}(\mathbf{s}) \cdot \widehat{\mathbb{1}_{\mathcal{A}}}(\mathbf{s}). \end{aligned} \tag{1}$$

The authors are with the Department of Electrical Communication Engineering, Indian Institute of Science, Bengaluru 560012, India (e-mail: vrameshwar@iisc.ac.in; nkashyap@iisc.ac.in).

We now recall the well-known proof of the fact that $2^n \cdot \widehat{\mathbb{1}_{W_i}}(\mathbf{s}) = K_i(w(\mathbf{s}))$ (see Chapter 5 in [1] for more details on Krawtchouk polynomials). Note that

$$2^n \cdot \widehat{\mathbb{1}_{W_i}}(\mathbf{s}) = \sum_{\mathbf{x}\in\{0,1\}^n:\ w(\mathbf{x})=i} (-1)^{\mathbf{x}\cdot\mathbf{s}}.$$

Now, the summation on the right side depends only on the weight $w(\mathbf{s})$, i.e., for any permutation of coordinates $\pi : \{0,1\}^n \to \{0,1\}^n$, it holds that

$$\sum_{\mathbf{x}\in\{0,1\}^n:\ w(\mathbf{x})=i} (-1)^{\mathbf{x}\cdot\pi(\mathbf{s})} = \sum_{\mathbf{x}\in\{0,1\}^n:\ w(\mathbf{x})=i} (-1)^{\pi(\mathbf{x})\cdot\pi(\mathbf{s})} = \sum_{\mathbf{x}\in\{0,1\}^n:\ w(\mathbf{x})=i} (-1)^{\mathbf{x}\cdot\mathbf{s}}.$$

In other words, we have that $\widehat{\mathbb{1}_{W_i}}(\mathbf{s}) = \widehat{\mathbb{1}_{W_i}}(\pi(\mathbf{s}))$. Hence, for $\mathbf{s}$ such that $w(\mathbf{s}) = j$, it suffices that we calculate $2^n \cdot \widehat{\mathbb{1}_{W_i}}(\mathbf{s}^\star)$, where $\mathbf{s}^\star = (s_1^\star, \ldots, s_n^\star)$ is such that $s_1^\star = \ldots = s_j^\star = 1$ and $s_{j+1}^\star = \ldots = s_n^\star = 0$. By a direct computation, it can be checked that $2^n \cdot \widehat{\mathbb{1}_{W_i}}(\mathbf{s}^\star) = \sum_{\ell=0}^{i} (-1)^\ell \binom{j}{\ell}\binom{n-j}{i-\ell} = 2^n \cdot \widehat{\mathbb{1}_{W_i}}(\mathbf{s})$. Plugging this back into (1) and simplifying, we obtain the expression in the theorem. □

As before, Theorem I.1 implies that if the Fourier coefficients $\widehat{\mathbb{1}_{\mathcal{A}}}(\mathbf{s})$ (or, the sum of Fourier coefficients at a fixed weight $\sum_{\mathbf{s}:\ w(\mathbf{s})=j} \widehat{\mathbb{1}_{\mathcal{A}}}(\mathbf{s})$) were available to us, we can easily compute the number of constrained words of a given weight.

## II. Weight Distribution of Constrained Codewords in Linear Codes

In this section, we briefly describe another useful computation that is facilitated by knowledge of the Fourier coefficients of the indicator function that a word belongs to a set of constrained sequences. Before we do so, we recall another property of Fourier transforms:

**Theorem II.1.** *Given functions $f, g : \{0,1\}^n \to \mathbb{R}$, the Fourier transform of $f \cdot g$ is the function $\widehat{f} \circledast \widehat{g}$, where*

$$(\widehat{f} \circledast \widehat{g})(\mathbf{s}) := \sum_{\mathbf{z}\in\{0,1\}^n} \widehat{f}(\mathbf{z})\widehat{g}(\mathbf{z}+\mathbf{s}) = 2^n \cdot (\widehat{f} \star \widehat{g})(\mathbf{s}), \quad \mathbf{s} \in \{0,1\}^n.$$

The calculation we wish to perform puts together the theses of Theorems III.1 of the paper and I.1 of the supplement. In particular, we ask for the number of codewords of a linear code $C$, which lie in a fixed set $\mathcal{A}$ and are of a given weight. We thus obtain Theorem II.2. For a given $\mathbf{v} \in \{0,1\}^n$, we use the notation $\mathbf{v}+C$ to denote the coset of $C$ to which $\mathbf{v}$ belongs. We let $a_{i,\mathcal{A}}(C)$ denote the number of constrained codewords of weight $i \in [0:n]$, which lie in the set $\mathcal{A}$ and in a linear code $C$.

**Theorem II.2.** *Given a linear code $C$ of blocklength $n$, we have that*

$$a_{i,\mathcal{A}}(C) = \frac{|C|}{2^n}\sum_{j=0}^{n} K_i^{(n)}(j) \sum_{\mathbf{s}:\ w(\mathbf{s})=j}\ \sum_{\mathbf{z}\in\mathbf{s}+C^\perp} \widehat{\mathbb{1}_{\mathcal{A}}}(\mathbf{z}).$$

*Proof.* We observe that

$$\begin{aligned} a_{i,\mathcal{A}}(C) &= \sum_{\mathbf{x}\in\{0,1\}^n} \mathbb{1}_{W_i}(\mathbf{x}) \cdot \mathbb{1}_{\mathcal{A}}(\mathbf{x}) \cdot \mathbb{1}_C(\mathbf{x}) \\ &= 2^n \cdot \sum_{\mathbf{s}\in\{0,1\}^n} \widehat{\mathbb{1}_{W_i}}(\mathbf{s}) \cdot \widehat{\mathbb{1}_{\mathcal{A}} \cdot \mathbb{1}_C}(\mathbf{s}), \end{aligned}$$

where the last equality above uses Plancherel's Theorem (see Theorem II.1 of the paper). Further, by employing Theorem II.1 to expand the last equality, we get that

$$\begin{aligned} a_{i,\mathcal{A}}(C) &= 2^n \cdot \sum_{\mathbf{s}\in\{0,1\}^n} \widehat{\mathbb{1}_{W_i}}(\mathbf{s}) \cdot \left(\widehat{\mathbb{1}_{\mathcal{A}}} \circledast \widehat{\mathbb{1}_C}\right)(\mathbf{s}) \\ &\overset{(a)}{=} \frac{|C|}{2^n} \cdot \sum_{\mathbf{s}\in\{0,1\}^n} K_i^{(n)}(w(\mathbf{s})) \sum_{\mathbf{z}\in\{0,1\}^n} \widehat{\mathbb{1}_{C^\perp}}(\mathbf{z}) \cdot \widehat{\mathbb{1}_{\mathcal{A}}}(\mathbf{s}+\mathbf{z}) \\ &= \frac{|C|}{2^n} \cdot \sum_{j=0}^{n} K_i^{(n)}(j) \sum_{\mathbf{s}:\ w(\mathbf{s})=j}\ \sum_{\mathbf{z}\in\mathbf{s}+C^\perp} \widehat{\mathbb{1}_{\mathcal{A}}}(\mathbf{z}), \end{aligned}$$

where equality (a) above uses the fact that $2^n \cdot \widehat{\mathbb{1}_{W_i}}(\mathbf{s}) = K_i^{(n)}(w(\mathbf{s}))$ and that $\widehat{\mathbb{1}_C}(\mathbf{s}) = \frac{|C|}{2^n} \cdot \mathbb{1}_{C^\perp}(\mathbf{s})$ (see the proofs of Theorems III.1 in the paper and I.1 in the supplement). □

Theorem II.2 could prove useful in the following context: consider the transmission of codewords of a linear code $C$ over an input-constrained binary-input memoryless symmetric (BMS) channel, which admits only binary constrained sequences that lie in the set $\mathcal{A}$ as inputs. Suppose

that the decoder being used is the maximum a-posteriori (MAP) (equivalently, the maximum likelihood (ML)) decoder of the linear code $\mathcal{C}$. By calculating the weight distribution of constrained codewords in a linear code $\mathcal{C}$ as above, it is possible to obtain an upper bound on the block error probability (via a union bounding argument), when the MAP decoder is used (see Chapter 1 of [2]).

## III. Obtaining MacWilliams' Identities for Linear Codes Via Theorem III.1 of the Paper

Consider the simple constraint that admits only sequences having a fixed weight $i \in [0:n]$, where $n$ is the blocklength of the code. Note that in this case, the set of constrained sequences is $\mathcal{A} = W_i$. By applying Theorem III.1 to this constraint, for a given linear code $\mathcal{C}$, we obtain the well-known MacWilliams' identities [3] for linear codes. We use the notation $a_i(\mathcal{C})$ for the number of codewords of weight $i \in [0:n]$ in $\mathcal{C}$, which equals $N(\mathcal{C}; W_i)$, following the notation of Theorem III.1 of the paper.

**Theorem III.1** (MacWilliams' identities)**.** *It is true that*

$$a_i(\mathcal{C}) = \frac{1}{|\mathcal{C}^\perp|}\sum_{j=0}^{n} K_i^{(n)}(j)\cdot a_j(\mathcal{C}^\perp).$$

*Proof.* The proof simply uses the fact that $\widehat{\mathbb{1}_{W_i}}(\mathbf{s}) = \frac{K_i^{(n)}(w(\mathbf{s}))}{2^n}$. By simplifying the summation in Theorem III.1 of the paper, and by using the fact that $|\mathcal{C}|\cdot|\mathcal{C}^\perp| = 2^n$, we obtain the required result. □

Further, it holds that the number of constrained codewords of weight $j$ obeys $a_{i,W_j} = \binom{n}{j}$, if $j = i$, and 0, otherwise.

## IV. Proof of Proposition III.1

*Proof.* Given the LP $\mathsf{Del}(n, d; \mathcal{A})$, defined by the objective function (Obj′) and the constraints (D1)–(D5), we define the new LP $\overline{\mathsf{Del}}(n, d)$ with the same objective function (Obj′) and using

the constraints (D1)–(D4) alone (excluding constraint (D5)). Thus, $\overline{\mathsf{Del}}(n,d)$ is given by:

$$\underset{f:\ \{0,1\}^n\to\mathbb{R}}{\text{maximize}} \quad \sum_{\mathbf{x}\in\{0,1\}^n} f(\mathbf{x}) \tag{Obj$'$}$$

subject to:

$$f(\mathbf{x}) \geq 0,\ \ \forall\ \mathbf{x}\in\{0,1\}^n, \tag{D1}$$

$$\widehat{f}(\mathbf{s}) \geq 0,\ \ \forall\ \mathbf{s}\in\{0,1\}^n, \tag{D2}$$

$$f(\mathbf{x}) = 0,\ \text{ if } 1\leq w(\mathbf{x})\leq d-1, \tag{D3}$$

$$f(0^n) \leq \text{val}(\mathsf{Del}(n,d)), \tag{D4}$$

It is therefore clear that for any $\mathcal{A}\subseteq\{0,1\}^n$, it holds that $\text{val}(\mathsf{Del}(n,d;\mathcal{A}))\leq\text{val}(\overline{\mathsf{Del}}(n,d))$. We now claim that $\text{val}(\overline{\mathsf{Del}}(n,d)) = (\text{val}(\mathsf{Del}(n,d)))^2$.

First, we shall show that the inequality in constraint (D4) in $\overline{\mathsf{Del}}(n,d)$ can be replaced with an equality. To see this, suppose that $f$ were an optimal solution to $\overline{\mathsf{Del}}(n,d)$, with $f(0^n) < \text{val}(\mathsf{Del}(n,d))$. Let $c>0$ be such that $c\leq\text{val}(\mathsf{Del}(n,d))-f(0^n)$. We then construct the function $\overline{f}:\{0,1\}^n\to\mathbb{R}$ such that $\overline{f}(0^n) = f(0^n)+c$, and $\overline{f}(\mathbf{x}) = f(\mathbf{x})$, for $\mathbf{x}\neq 0^n$. It can then easily be verified that $\overline{f}$ satisfies constraints (D1), (D3) and (D4). Furthermore, $\overline{f}$ satisfies (D2) also, since by linearity of the Fourier transform, for any $\mathbf{s}\in\{0,1\}^n$, it holds that

$$\begin{aligned}\widehat{(\overline{f})}(\mathbf{s}) &= \widehat{f}(\mathbf{s}) + c\cdot\widehat{\mathbb{1}_{\{0^n\}}}(\mathbf{s})\\ &= \widehat{f}(\mathbf{s}) + \frac{c}{2^n}\geq 0.\end{aligned}$$

Hence, $\overline{f}$ is a feasible solution to $\overline{\mathsf{Del}}(n,d)$, with $\text{val}(\overline{f}) = \sum_{\mathbf{x}\in\{0,1\}^n} f(\mathbf{x}) + c > \text{val}(f)$, which contradicts the optimality of $f$. Hence, any optimal solution to $\overline{\mathsf{Del}}(n,d)$ must be such that (D4) is satisfied with an equality, and we can thus replace the inequality in (D4) with an equality.

Now, in order to prove that $(\text{val}(\overline{\mathsf{Del}}(n,d)))^{1/2} = \text{val}(\mathsf{Del}(n,d))$, it suffices to observe that any feasible solution $f$ of $\mathsf{Del}(n,d)$ yields a feasible solution $\text{val}(\mathsf{Del}(n,d))\cdot f$, to $\overline{\mathsf{Del}}(n,d)$ (with the inequality in (D4) changed to an equality). Likewise, any feasible solution $f$ of $\overline{\mathsf{Del}}(n,d)$ yields a feasible solution $\frac{f}{\text{val}(\mathsf{Del}(n,d))}$, to $\mathsf{Del}(n,d)$. Owing to this bijection, we obtain that $\text{val}(\overline{\mathsf{Del}}(n,d)) =$

$\mathrm{val}(\mathsf{Del}(n,d))^2$.

Using the fact that $\mathrm{val}(\mathsf{Del}(n,d;\mathcal{A})) \leq \mathrm{val}(\overline{\mathsf{Del}}(n,d))$, we obtain the statement of the proposition. □

## V. An Upper Bound on $\mathrm{val}(\mathsf{Del}(n,d;\mathcal{A}))$

In this section, we derive an upper bound on the optimal value $\mathrm{val}(\mathsf{Del}(n,d;\mathcal{A}))$ of our LP, in the following lemma that is essentially a formulation of the dual LP. We believe that the lemma will serve useful in the derivation of asymptotic (as the blocklength goes to infinity) upper bounds on the rate-distance tradeoff for constrained codes. We abbreviate $\mathrm{val}(\mathsf{Del}(n,d))$ as $v$ and $\mathrm{val}(\mathsf{Del}(n,d;\mathcal{A}))$ as $v_{\mathcal{A}}$.

**Lemma V.1.** *Let $\beta : \{0,1\}^n \to \mathbb{R}$ be a function that satisfies $\widehat{\beta}(\mathbf{s}) \geq 0$, for all $\mathbf{s} \in \{0,1\}^n$, and $\sum_{\mathbf{x}} \beta(\mathbf{x}) = 1$. Then,*

$$v_{\mathcal{A}} \leq 2^n \cdot \left[\beta(0^n)\cdot \min\{v, |\mathcal{A}|\} + 2^n \cdot \sum_{\mathbf{x}:\ w(\mathbf{x})\geq d} \beta(\mathbf{x}) \cdot (\mathbb{1}_{\mathcal{A}} \star \mathbb{1}_{\mathcal{A}})(\mathbf{x})\right].$$

*Proof.* Consider any function $\lambda : \{0,1\}^n \to [0,\infty)$. Now, observe that for any feasible solution $f$ of $\mathsf{Del}(n,d;\mathcal{A})$, we have that

$$\begin{aligned}
\lambda(0^n)\cdot \widehat{f}(0^n) &\overset{(a)}{\leq} \sum_{\mathbf{x}\in\{0,1\}^n} \lambda(\mathbf{x}) \cdot \widehat{f}(\mathbf{x}) \\
&\overset{(b)}{=} 2^n \cdot \sum_{\mathbf{s}\in\{0,1\}^n} \widehat{\lambda}(\mathbf{s}) \cdot \frac{f(\mathbf{s})}{2^n} \\
&\overset{(c)}{=} \sum_{\substack{\mathbf{s}:\ \mathbf{s}\,=\,0^n \text{ or} \\ w(\mathbf{s})\geq d}} \widehat{\lambda}(\mathbf{s}) \cdot f(\mathbf{s}) \\
&\overset{(d)}{\leq} \widehat{\lambda}(0^n)\cdot \min\{v, |\mathcal{A}|\} + 2^n \cdot \sum_{\mathbf{s}:\ w(\mathbf{s})\geq d} \widehat{\lambda}(\mathbf{s}) \cdot (\mathbb{1}_{\mathcal{A}} \star \mathbb{1}_{\mathcal{A}})(\mathbf{s}),
\end{aligned}$$

where (a) holds since $\lambda, \widehat{f} \geq 0$, (b) holds by an application of Plancherel's Theorem, along with the fact that $\widehat{(\widehat{f})} = 2^{-n}\cdot f$. Next, (c) is true since $f$ satisfies (D3) and (d) holds since $f$ satisfies (D4) and (D5), and since $2^n \cdot (\mathbb{1}_{\mathcal{A}} \star \mathbb{1}_{\mathcal{A}})(0^n) = |\mathcal{A}|$.

Moreover, we have that $\mathrm{val}(f) = \sum_{\mathbf{x}\in\{0,1\}^n} f(\mathbf{x}) = 2^n \cdot \widehat{f}(0^n)$, and that $\lambda(0^n) = \sum_{\mathbf{s}\in\{0,1\}^n} \widehat{\lambda}(\mathbf{s})$, by the definition of the Fourier transform. Putting everything together, we obtain that for any feasible $f$ of $\mathsf{Del}(n,d;\mathcal{A})$, it holds that

$$\mathrm{val}(f) \leq \frac{2^n}{\sum_{\mathbf{s}} \widehat{\lambda}(\mathbf{s})} \cdot \left[\widehat{\lambda}(0^n) \cdot \min\{v, |\mathcal{A}|\} + 2^n \cdot \sum_{\mathbf{s}\colon\ w(\mathbf{s})\geq d} \widehat{\lambda}(\mathbf{s}) \cdot (\mathbb{1}_{\mathcal{A}} \star \mathbb{1}_{\mathcal{A}})(\mathbf{s})\right].$$

Finally, by substituting $\beta$ as $\widehat{\lambda}$ and ensuring that $\sum_{\mathbf{x}} \widehat{\beta}(\mathbf{x}) = 1$, we obtain the thesis of the lemma. □

## VI. Proof of Lemma IV.3

*Proof.* We have that

$$\begin{aligned} 2^n \cdot \widehat{\mathbb{1}_{C_z^p}}(\mathbf{s}) &= \sum_{\mathbf{x}\in\{0,1\}^n\colon\ \mathbf{x}\in C_z^p} (-1)^{\mathbf{x}\cdot\mathbf{s}} \\ &= \sum_{\mathbf{x}_1\in\{0,1\}^{n/p}\colon\ w(\mathbf{x})=z} \cdots \sum_{\mathbf{x}_p\in\{0,1\}^{n/p}\colon\ w(\mathbf{x})=z} (-1)^{\mathbf{x}\cdot\mathbf{s}_1} \ldots (-1)^{\mathbf{x}\cdot\mathbf{s}_p} \\ &= \prod_{\ell=1}^{p} \left( \sum_{\mathbf{x}_\ell\in\{0,1\}^{n/p}\colon\ w(\mathbf{x})=z} (-1)^{\mathbf{x}\cdot\mathbf{s}_\ell} \right). \end{aligned}$$

Now, by following a line of argument similar to that in the proof of Theorem I.1 in Appendix I, we obtain that for any $\ell \in [p]$, the value of the inner summand depends on $\mathbf{s}_\ell$ only via its weight. In other words, it holds that for any $\ell \in [p]$,

$$\sum_{\mathbf{x}_\ell\in\{0,1\}^{n/p}\colon\ w(\mathbf{x})=z} (-1)^{\mathbf{x}\cdot\mathbf{s}_\ell} = \sum_{\mathbf{x}_\ell\in\{0,1\}^{n/p}\colon\ w(\mathbf{x})=z} (-1)^{\mathbf{x}\cdot\tilde{\mathbf{s}}_\ell},$$

where $\tilde{\mathbf{s}}_\ell = (\underbrace{1,1,\ldots,1}_{w(\mathbf{s}_\ell)\text{ such}},0,0,\ldots,0)$. By direct calculations, it holds that the sum in right-hand side of the expression above equals $K_z^{(n/p)}(w(\mathbf{s}_\ell))$. □

## VII. Proof of Lemma IV.5

*Proof.* To prove the first recurrence relation, we write

$$\widehat{\mathbb{1}_{S^d}}^{(n)}(\mathbf{s}) = \frac{1}{2^n} \cdot \sum_{\mathbf{x}\in S^d} (-1)^{\mathbf{x}\cdot\mathbf{s}}$$
$$= 2^{-n} \cdot \Big( \#\{x^n \in S^d : \ w_{\mathbf{s}}(x^n) \text{ is even}\} - \#\{x^n \in S^d : \ w_{\mathbf{s}}(x^n) \text{ is odd}\} \Big). \tag{2}$$

Now, observe that

$$\#\{x^n \in S^d : \ w_{\mathbf{s}}(x^n) \text{ is even}\} = \#\{x^n \in S^d : \ w_{\mathbf{s}}(x^n) \text{ is even and } x_1 = 0\} +$$
$$\#\{x^n \in S^d : \ w_{\mathbf{s}}(x^n) \text{ is even and } x_1 = 1\}$$
$$\stackrel{(a)}{=} \#\{x_2^n \in S^d : \ w_{s_2^n}(x_2^n) \text{ is even}\} +$$
$$\#\{x^n \in S^d : \ w_{\mathbf{s}}(x^n) \text{ is even and } x_1^{(d+1)} = 10^d\}$$
$$= \#\{x_2^n \in S^d : \ w_{s_2^n}(x_2^n) \text{ is even}\} + \#\{x_{d+2}^n \in S^d : \ w_{s_{d+2}^n}(x^n) \text{ is even}\}, \tag{3}$$

where (a) holds because $s_1 = 0$ and from the fact that the $(d, \infty)$-RLL constraint requires that $x_2^{d+1} = 0^d$, if $x_1 = 1$. Similarly, we obtain that

$$\#\{x^n \in S^d : \ w_{\mathbf{s}}(x^n) \text{ is odd}\} = \#\{x_2^n \in S^d : \ w_{s_2^n}(x_2^n) \text{ is odd}\} + \#\{x_{d+2}^n \in S^d : \ w_{s_{d+2}^n}(x^n) \text{ is odd}\}. \tag{4}$$

Now, observe that

$$\widehat{\mathbb{1}_{S^d}}^{(n-1)}(s_2^n) = 2^{-(n-1)} \cdot \Big( \#\{x_2^n \in S^d : \ w_{s_2^n}(x_2^n) \text{ is even}\} - \#\{x_2^n \in S^d : \ w_{s_2^n}(x_2^n) \text{ is odd}\} \Big) \tag{5}$$

and that

$$\widehat{\mathbb{1}_{S^d}}^{(n-d-1)}(s_{d+2}^n) = 2^{-(n-d-1)} \cdot \Big( \#\{x_{d+2}^n \in S^d : \ w_{s_{d+2}^n}(x_{d+2}^n) \text{ is even}\} -$$
$$\#\{x_{d+2}^n \in S^d : \ w_{s_{d+2}^n}(x_{d+2}^n) \text{ is odd}\} \Big). \tag{6}$$

Substituting (3) and (4) in (2) and using (5) and (6), we get the first recurrence relation. The second recurrence relation is also proved by similar arguments. □

## REFERENCES

[1] F. J. MacWilliams and N. J. A. Sloane, *The Theory of Error-Correcting Codes*, 2nd ed. North-Holland, 1978.

[2] T. Richardson and R. Urbanke, *Modern Coding Theory*. Cambridge University Press, 2008.

[3] J. MacWilliams, "A theorem on the distribution of weights in a systematic code," *The Bell System Technical Journal*, vol. 42, no. 1, pp. 79–94, 1963.
